# Supplementary material for: Picosecond Dynamic Heterogeneity, Hopping and Johari-Goldstein Relaxation in Glassforming Liquids
Source: arXiv:1310.6375 source file (2014-06-30)
Supplement: Supplementary file 1 [file TwoStateV3_SI.pdf]

**Experimental Procedure**

All samples were purchased from Sigma-Aldrich [1] fully hydrogenated, and of ≥ 99% purity. Except o-terphenyl (OTP), samples were used without further purification. OTP, 99%, was recrystallized in methanol several times to purify it further as relaxation of OTP is known to be affected by small traces of impurities. After purification, OTP was kept in vacuum oven at 80 °C for several days to remove residual solvent.

Samples were loaded in annular sample can of thickness 0.1mm and the estimated transmission was 92% for all the samples. Higher transmission minimizes multiple scattering effects and the annular sample minimizes q-dependent absorption changes.

Neutron scattering from all the samples was measured with the Disk Chopper Spectrometer (DCS) installed at the NG4 guide at the NIST Center for Neutron Research [2]. The neutron wavelength was set at 4 Å, which corresponded to a momentum transfer (q) range of 0.2 $Å^{-1}$ to 2.8 $Å^{-1}$. The DCS instrument has 994 detectors to cover this q range; data was binned in the step of 0.1$Å^{-1}$ in order to improve statistics of measured S(q,ω). In order to check the statistics, a binning step of 0.2 $Å^{-1}$ was also used. This binning step was discarded later as no significant differences were observed between the two data sets. The instrumental resolution was about 0.19 meV and the maximum energy transfer was about 4.5 meV. More details of the instrument can be found in Ref.2.

As the neutron flux is relatively high at 4Å wavelength, data at each temperature was obtained within (3 to 6) h and had good statistics. An example of typical data can be seen in Fig.1 where we have plotted raw data for all glass formers used in this study at representative temperatures.

Some of the glassformers used tend to crystallize, so experiments were performed on cooling from the high temperature to avoid potential artifacts from crystal nucleation at low temperature. We ensured that there was no sign of crystallization even on reheating, when crystal nuclei would have grown if they had seeded at low temperature. Absence of crystallization was confirmed by noting an absence of Bragg peaks in plots of scattered intensity vs q.

The data sets were corrected for i) background from empty can ii) dark count background (with neutron beam off) and iii) detector efficiencies by measuring a vanadium standard. All the data files were reduced using the mslice utility under DAVE software available at NIST [3].

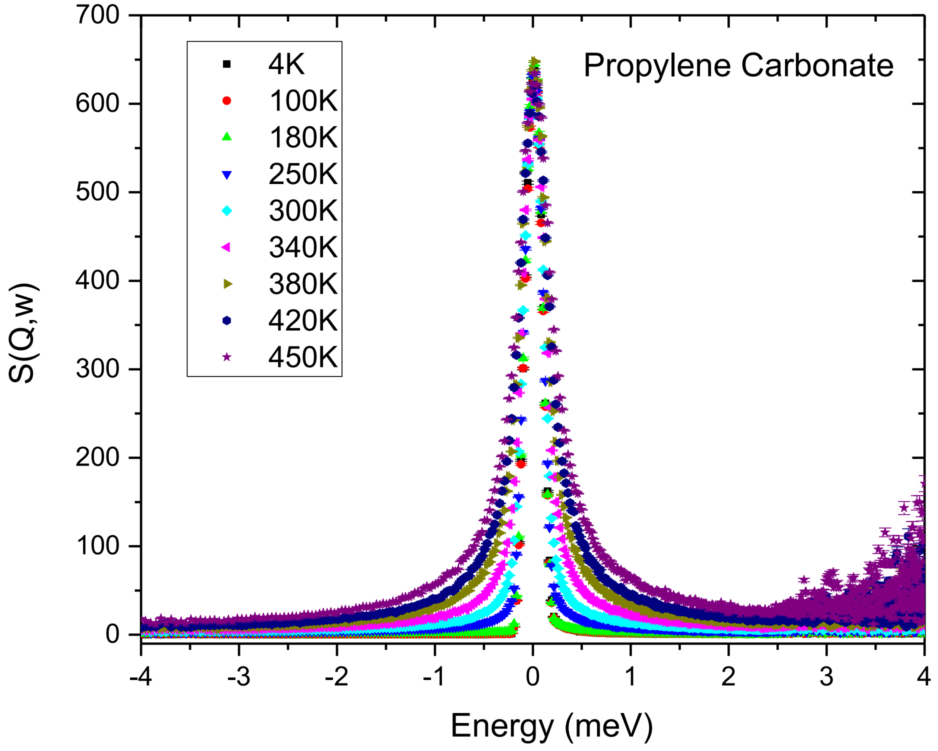
Propylene Carbonate
4K
100K
180K
250K
300K
340K
380K
420K
450K
S(Q,w)
Energy (meV)
700
600
500
400
300
200
100
0
-4
-3
-2
-1
0
1
2
3
4

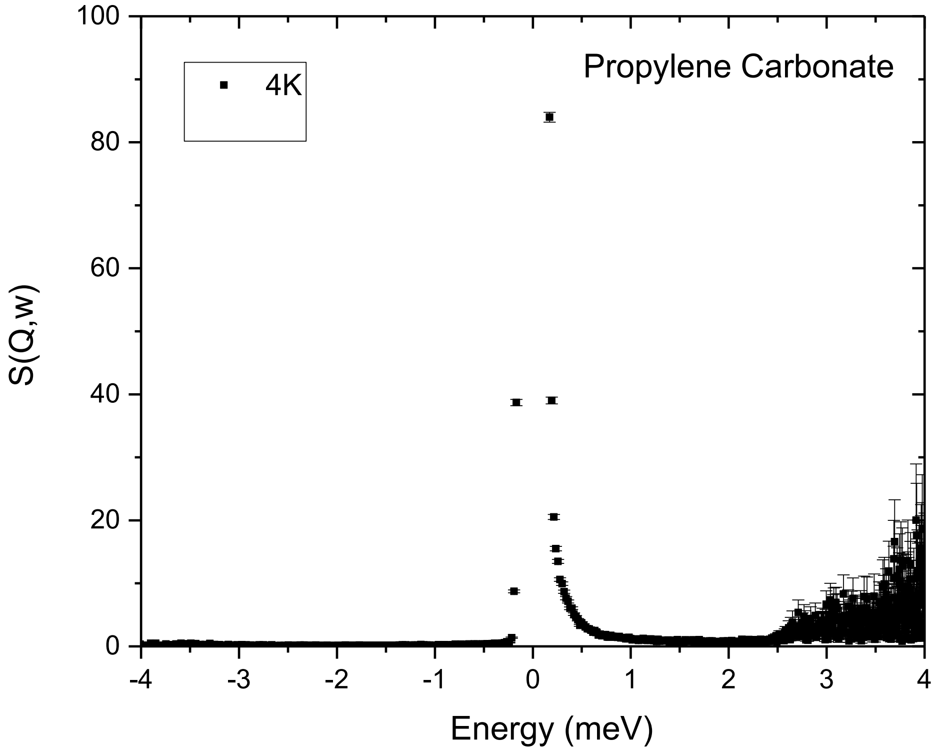
Propylene Carbonate
4K
S(Q,w)
Energy (meV)
100
80
60
40
20
0
-4
-3
-2
-1
0
1
2
3
4

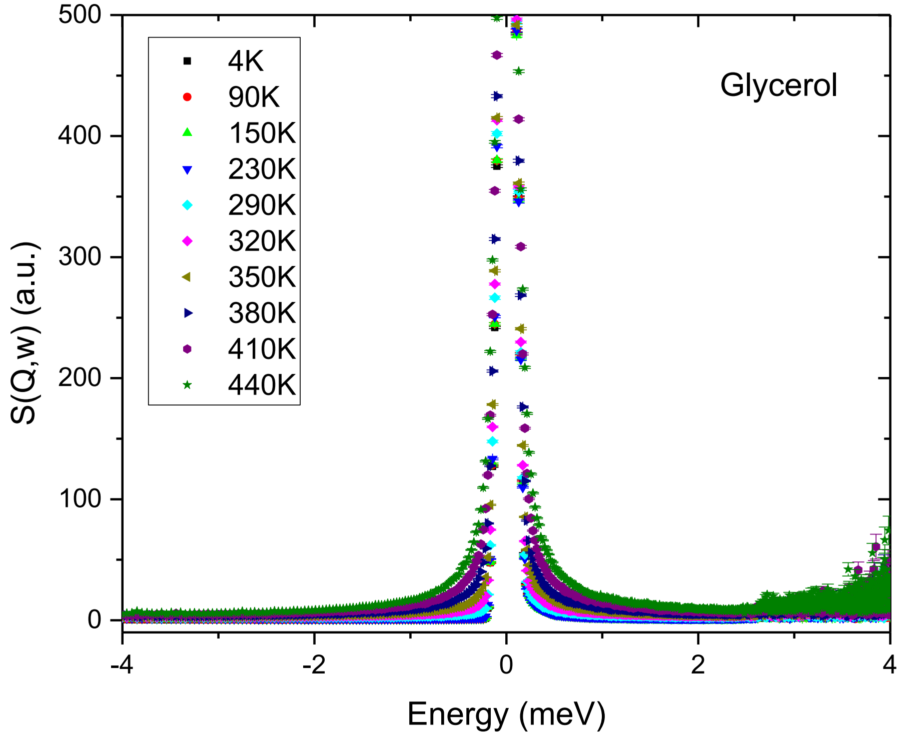

Glycerol
4K
90K
150K
230K
290K
320K
350K
380K
410K
440K
S(Q,w) (a.u.)
Energy (meV)
500
400
300
200
100
0
-4
-2
0
2
4


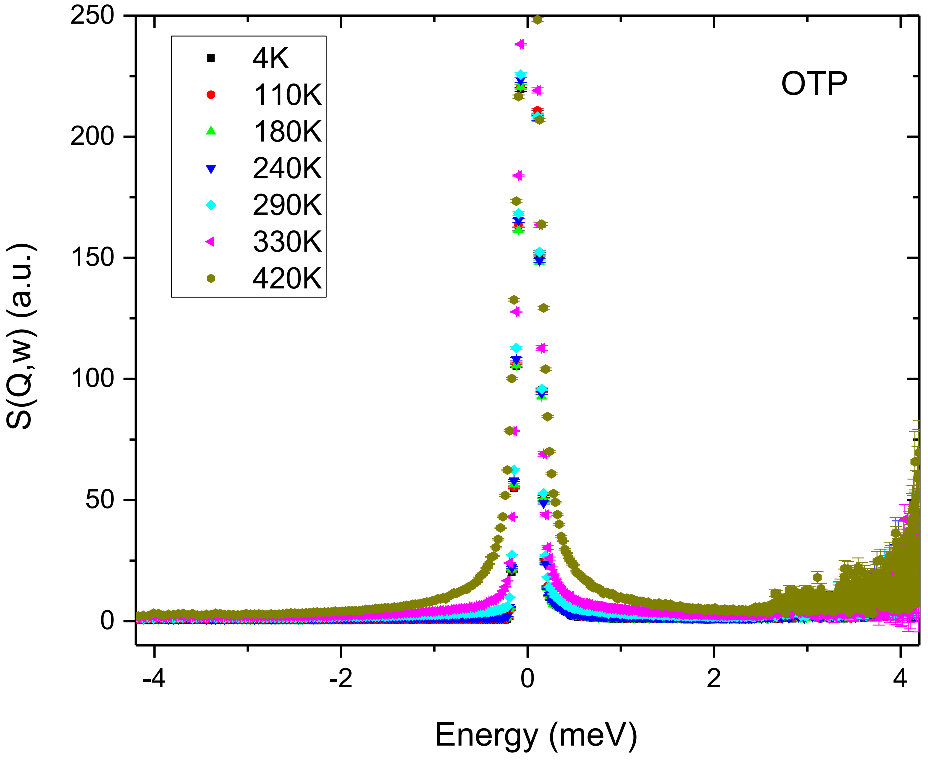

OTP
4K
110K
180K
240K
290K
330K
420K
S(Q,w) (a.u.)
Energy (meV)
250
200
150
100
50
0
-4
-2
0
2
4

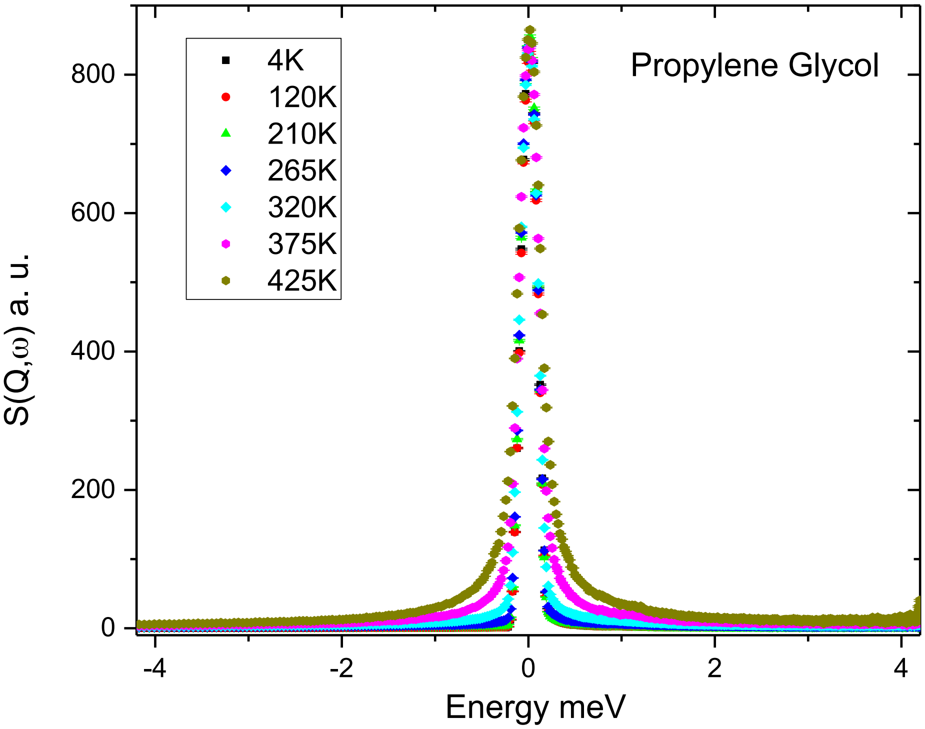
Propylene Glycol
4K
120K
210K
265K
320K
375K
425K
S(Q,ω) a. u.
Energy meV
0
200
400
600
800
-4
-2
0
2
4

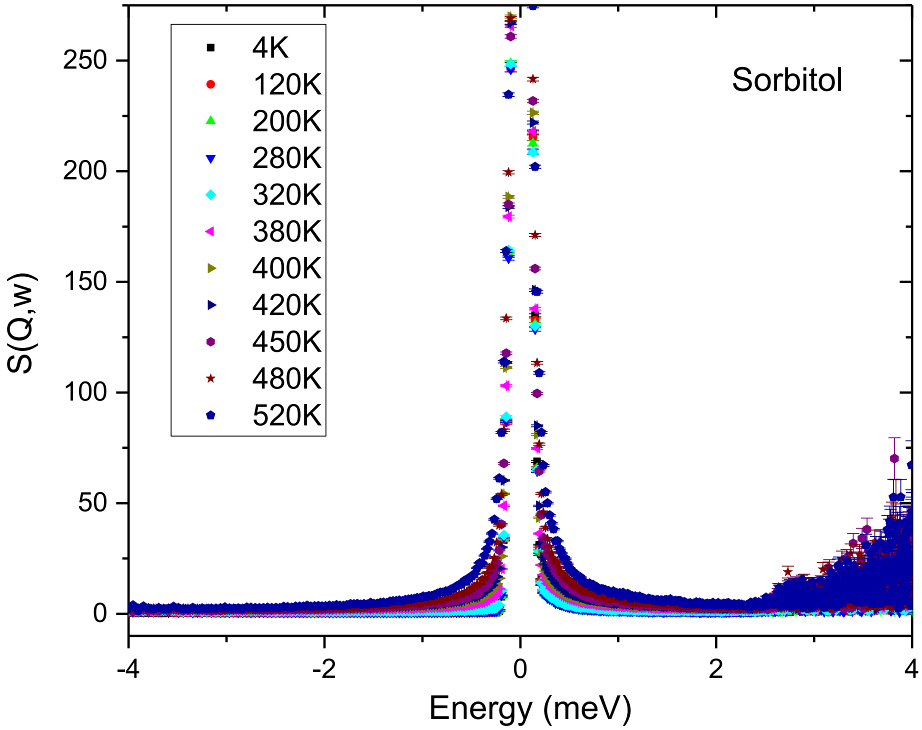
Sorbitol
4K
120K
200K
280K
320K
380K
400K
420K
450K
480K
520K
S(Q,w)
Energy (meV)
0
50
100
150
200
250
-4
-2
0
2
4

***Figure S1:*** *Quasi-elastic representative data for all glass formers at selected temperatures. Data has been summed for Q values between 0.5Å$^{-1}$ and 1.0Å$^{-1}$ and for the sake of clarity peak heights has been normalized.*

## Fourier Transform of S(q,ω)

The neutron scattering measurements provided dynamic scattering functions S(q,ω) in the frequency domain. DAVE software was used to Fourier transform the experimental data from frequency to time domain in order to give the intermediate scattering function, F(q,t). The real part of the Fourier transformed data was used to calculate F(q,t), and no filtering options were used as they were not found necessary. See Ref. 3, references therein, and www.ncnr.nist.gov/DAVE for more details.

Deconvolution of the scattering data was performed in the time domain. In the frequency domain, measured data is a combination of true dynamic scattering function convolved with instrument resolution –

$$S_{expt}(q,\omega) = S_{true}(q,\omega) \otimes R(q,\omega) \qquad (1)$$

where R(Q,ω) is instrumental resolution. When the data is transformed to the time domian, we obtain

$$F_{expt}(q,t) = F_{true}(q,t) \times R(q,t) \qquad (2)$$

and, the deconvolved intermediate scattering function can be calculated directly as $F_{true}$= $F_{expt}$ /R.

In all cases, S(q,ω) of the material at 4 K was used as the resolution function R(q,ω). Scattering from samples at 4 K was compared with standard vanadium, and found to contain no broadening from, e.g. methyl group rotation etc., so these data sets were deemed acceptable for normalizing F(q,t). The fact that coherent scattering is only about 5% of the total scattering in these samples amelioriates the complications arising from coherent scattering when base temperature data is used as resolution for higher temperatures.

Noise is propagated in the Fourier transform operation, and additional errors can arise through truncation and course sampling intervals. These factors are taken into account and standard uncertainties are calculated by the DAVE software. An example of transformed data, along with standard deviations, is given in Table S1. The errors are typically too small

to be appreciated in a graphical representation. Small error bars in time domain data show systematic errors are not significant in data handling.

Table S1: Values and Standard Deviation for ISF of PG at 320 K

| Q | F(q,t) | S. Dev. F(q,t) | -ln(F) | S.Dev. -ln(F) |
|---|---|---|---|---|
| 0.2 | 0.940000003 | 0.004852096 | 0.0618754 | 0.0103237 |
| 0.3 | 0.929999993 | 0.002748453 | 0.0725707 | 0.00591067 |
| 0.4 | 0.912999999 | 0.001461095 | 0.0910194 | 0.003200648 |
| 0.5 | 0.884999676 | 0.00140587 | 0.122168 | 0.003177111 |
| 0.6 | 0.851999789 | 0.001101884 | 0.160169 | 0.002586585 |
| 0.7 | 0.81900016 | 0.001403112 | 0.199671 | 0.003426406 |
| 0.8 | 0.787000024 | 0.001358494 | 0.239527 | 0.003452338 |
| 0.9 | 0.76099994 | 0.001520067 | 0.273122 | 0.003994927 |
| 1 | 0.730999868 | 0.001349867 | 0.313342 | 0.003693211 |
| 1.1 | 0.699999961 | 0.001375323 | 0.356675 | 0.003929499 |
| 1.2 | 0.671999959 | 0.001526078 | 0.397497 | 0.004541906 |
| 1.3 | 0.64799973 | 0.001315289 | 0.433865 | 0.004059542 |
| 1.4 | 0.622000116 | 0.001385151 | 0.474815 | 0.00445387 |
| 1.5 | 0.597000099 | 0.001193667 | 0.515838 | 0.003998889 |
| 1.6 | 0.566000114 | 0.00135814 | 0.569161 | 0.00479909 |
| 1.7 | 0.537000099 | 0.001322148 | 0.621757 | 0.004924211 |
| 1.8 | 0.504000005 | 0.001304046 | 0.685179 | 0.005174798 |
| 1.9 | 0.481000004 | 0.001284389 | 0.731888 | 0.005340506 |
| 2 | 0.459000032 | 0.001432315 | 0.778705 | 0.006241046 |
| 2.1 | 0.427000113 | 0.001289268 | 0.850971 | 0.006038742 |
| 2.2 | 0.399999893 | 0.000947523 | 0.916291 | 0.004737626 |
| 2.3 | 0.381999874 | 0.001257872 | 0.962335 | 0.006585745 |
| 2.4 | 0.358000821 | 0.000909905 | 1.02722 | 0.005083267 |
| 2.5 | 0.333000929 | 0.000928785 | 1.09961 | 0.005578286 |

**Fitting $F_s(q,t)$**

All $F_s(q,t)$ data were fitted to a double-Gaussian model as given by Eq. 1 of the main text. From the behavior of the fitting we conclude that the motion associated with $\sigma_{LC}$ is largely intermolecular in nature, and that multiple scattering does not significantly affect our fit results. Contributions to $F_s$ from multiple scattering events and from molecular relaxation can be separated based on their q-dependence. The former are most dominant at low q, but diminish with increasing q, while the latter have the opposite q-dependence. Figure S2a shows $-\ln(F_s)$ for glycerol at t= 1 ps and the lowest q values obtained. We observe that, for $q \leq 0.3$ Å$^{-1}$, $-\ln(F_s)$, drops with decreasing q. This is unphysical for an incoherent intermediate scattering function, and the drop in $-\ln(F_s)$ is a manifestation of multiple scattering. The fact that $-\ln(F_s)$ has a positive q-dependence for $q > 0.3$ Å$^{-1}$, indicates that the contribution from multiple scattering is less than that from single scattering events at these higher q values. Since multiple scattering drops off quickly at higher q values [4], while the singly scattered quasielastic neutron flux rises rapidly with q, the influence of multiple scattering quickly becomes inconsequential at higher q values. We verified that multiple scattering did not significantly impact the fit parameters we obtain this by noting that there was no change in fit parameter values when varying the low-q cutoff for data points to fit, as long as $q_{cutoff} > 0.3$ Å$^{-1}$. Thus, we discarded the two data points at the lowest q values (0.2 and 0.3 Å$^{-1}$) for all samples.

Panels b-c of Figure S2 show the sensitivity of fits to variation in each of the fit parameters. All data are $F_s(q,1\text{ ps})$ in glycerol at 260 K. We have plotted the data at the lowest two q values, although these are not used in the fits. The solid black line is the best fit to the data in each case, and the dashed blue lines show variation in the fit when varying the indicated parameter by ± 3 standard deviations. We note that variation in $\sigma_{TC}$ and $\sigma_{LC}$ impact completely different q regions, with variations in $\sigma_{LC}$ impacting only $q \leq 1$ Å$^{-1}$. This behavior is due to the pronounced separation between $\sigma_{TC}$ and $\sigma_{LC}$ values, and similar behavior is observed for fitting in each of the materials. We note that the peak in the static structure factor ($q_{max}$) is approximately 1.4 Å$^{-1}$ for each of these materials, so $\sigma_{LC}$ fit values pertain only to scattering at $q < q_{max}$, which is due primarily to intermolecular motion.

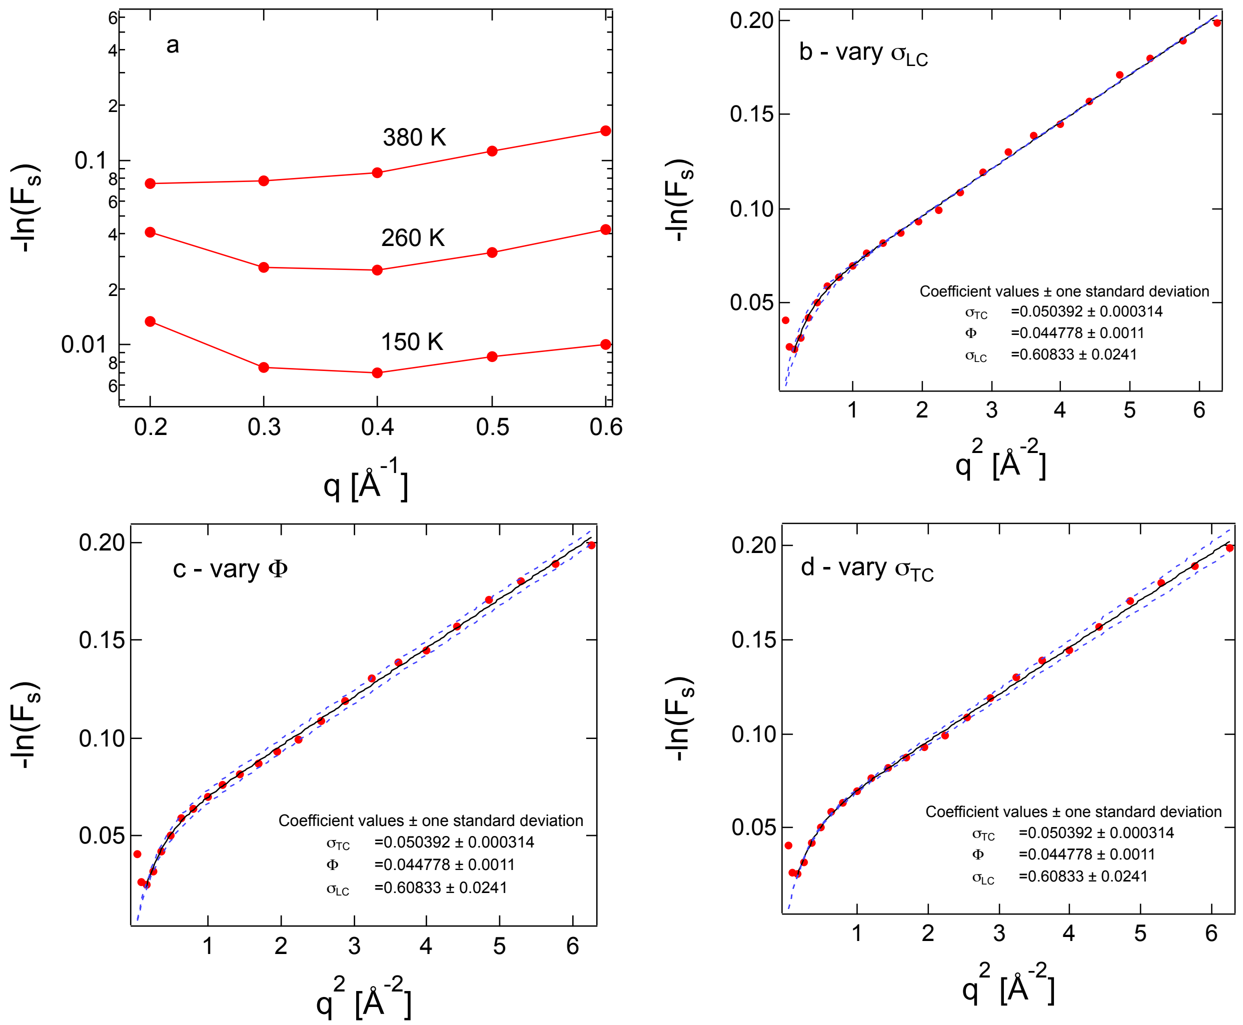


***Figure S2:*** *a) Lowest q points of F(q,1 ps) in glycerol at temperatures indicated. Lowest two points are clearly influenced by multiple scattering, and are omitted when fitting. b-d) Effects on overall fit of varying parameters. Solid black line is the best fit to the data, and the blue dashed lines are the fits obtained by varying the indicated parameter ±3 standard deviations. b) Effect of varying* $\sigma_{TC}$*, c) Effect of varying* $\Phi$*, d) effect of varying* $\sigma_{LC}$*.*

Figures S3 and S4 present fits for all $F_s$ data used. Temperatures at which data were obtained are given in Table S2. Data from lowest temperatures appear lowest on the plots. We note that the fits are excellent in essentially all cases.

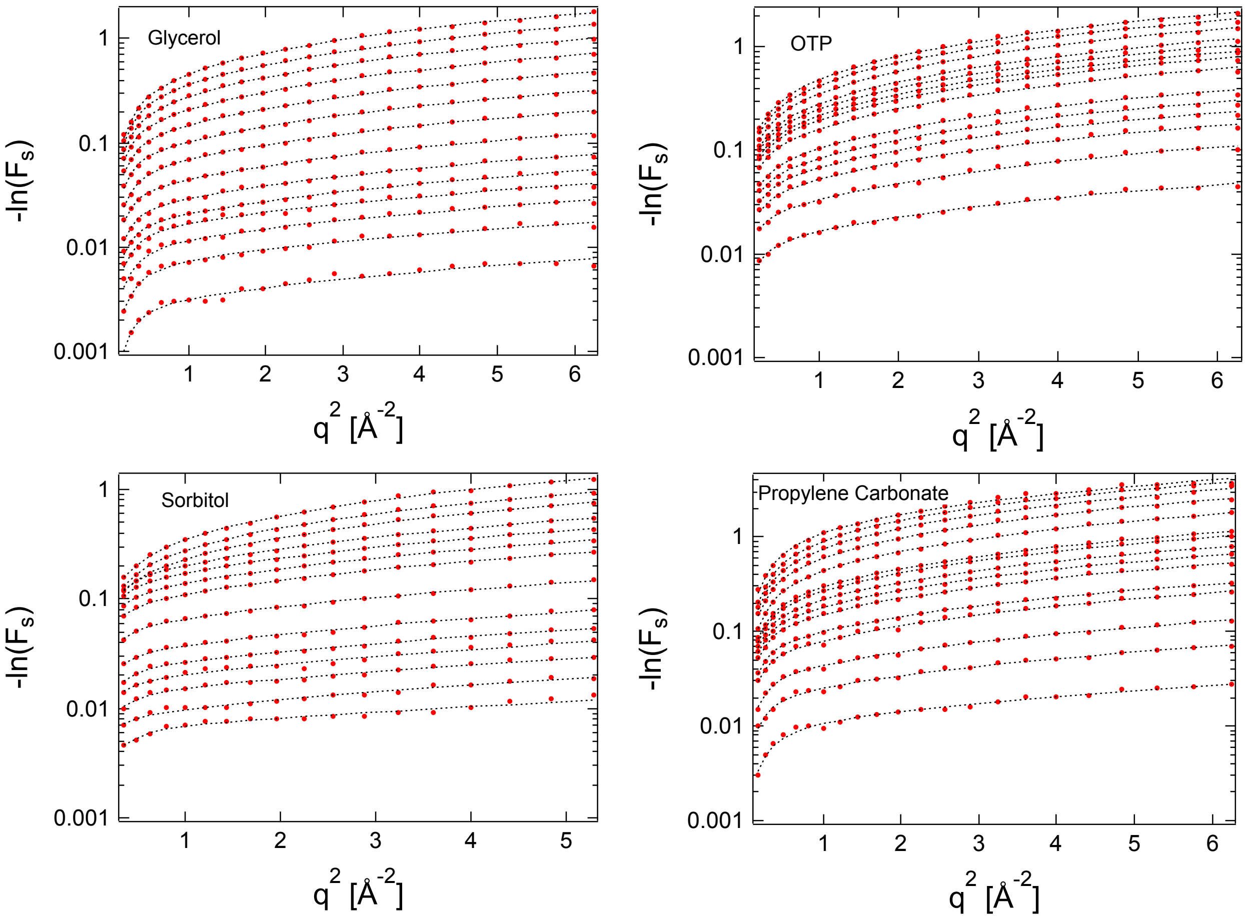


***Figure S3:*** *F(q,t=1ps) data obtained from S(q,ω) as described above. Dashed lines are fits to Equation (1) in the main text.*

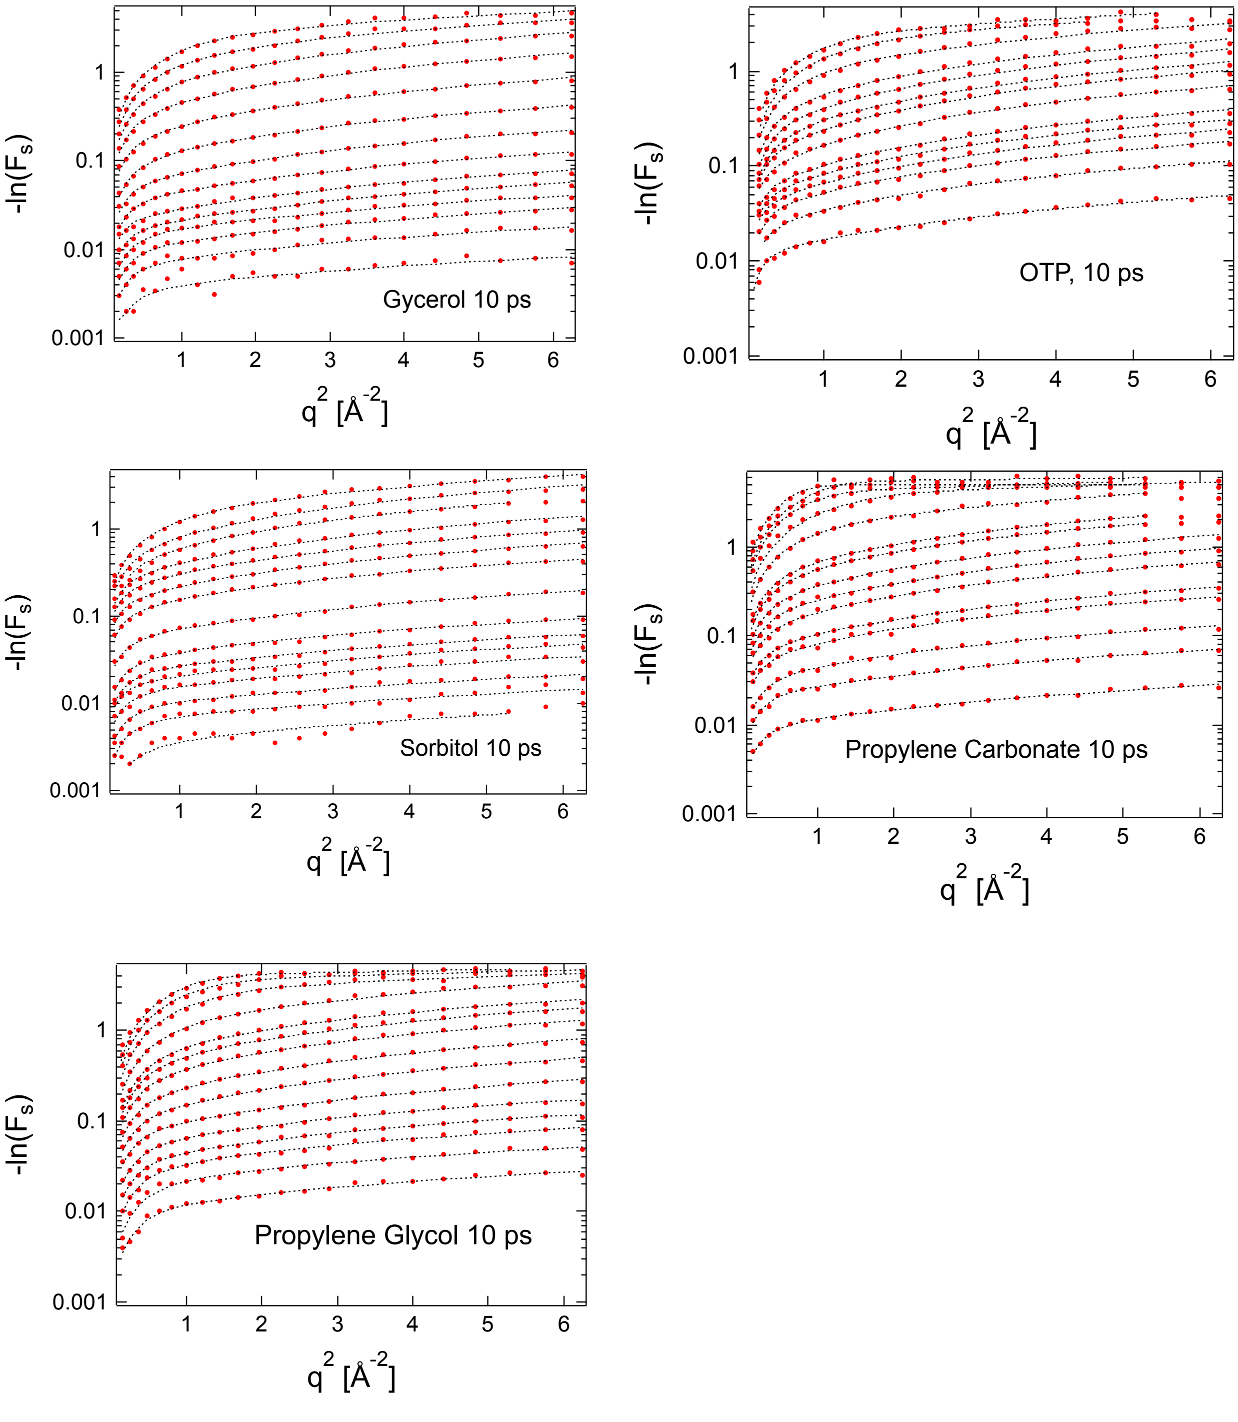


***Figure S4:*** *F(q,t=10 ps) data obtained from S(q,ω) as described above. Dashed lines are fits to Equation (1) in the main text.*

**Table S2 – Temperatures [K] at which data are recorded in Figures S3 and S4**

| PC | PG | Glycerol | OTP | Sorbitol |
|---|---|---|---|---|
| 60 | 60 | 60 | 70 | 60 |
| 100 | 90 | 90 | 110 | 90 |
| 140 | 120 | 120 | 150 | 120 |
| 160 | 150 | 150 | 180 | 160 |
| 180 | 180 | 180 | 210 | 200 |
| 193 | 210 | 200 | 240 | 240 |
| 206 | 240 | 230 | 270 | 280 |
| 220 | 265 | 260 | 290 | 320 |
| 240 | 290 | 290 | 300 | 360 |
| 250 | 307 | 320 | 315 | 380 |
| 300 | 320 | 350 | 330 | 400 |
| 340 | 350 | 380 | 360 | 420 |
| 380 | 375 | 410 | 390 | 450 |
| 420 | 400 | 440 | 420 | 480 |
| 450 | 425 | | | 520 |

**References:**


[1] The identification of commercial products does not imply endorsement by the National Institute of Standards and Technology nor does it imply that these are the best for the purpose.

[2] J.R.D. Copley and J.C. Cook, Chem. Phys. 292, 477 (2003).

[3] R.T. Azuah, L.R. Kneller, Y. Qiu, P.L.W. Tregenna-Piggott, C.M. Brown, J.R.D. Copley, and R.M. Dimeo, J. Res. Natl. Inst. Stan. Technol. 114, 341 (2009).

[4] J. Wuttke, I. Chang, O.G. Randl, F. Fujara, and W. Petry, Physical Review E 54, 5364 (1996).
